# Supplementary material for: Say It Another Way: Auditing LLMs with a User-Grounded Automated Paraphrasing Framework
Source: arXiv:2505.03563 source file (2026-11-16)
Supplement: Supplementary file 1 [file app_characters.tex]

\section{Context characteristics} \label{annex:char}
Table \ref{tab:char} presents characteristics on the context length for the Gender Identity Subset, that was used for the paraphrasing module.
\begin{table}[H]
\centering
\begin{tabular}{lcc}
\toprule
\textbf{Context Type} & \textbf{Avg. Length} & \textbf{Range} \\
\midrule
Amb & $103 \pm 29$ & 53--166 \\
Dis & $275 \pm 55$ & 173--378 \\
\bottomrule
\end{tabular}
\caption{\centering Character length statistics for different context types.}
\label{tab:char}
\end{table}
