# Supplementary material for: Say It Another Way: Auditing LLMs with a User-Grounded Automated Paraphrasing Framework
Source: arXiv:2505.03563 source file (2026-11-16)
Supplement: Supplementary file 2 [file app_violin.tex]

\section{Thresholds} \label{annex:thresh}
Figures \ref{fig:violin-sbert}, \ref{fig:violin-bert}, \ref{fig:violin-rouge}, \ref{fig:violin-ppl} present the distribution of similarity metrics and perplexity ratio across paraphrase types.

\begin{figure*}[t]
\centering
        \includegraphics[width=\linewidth]{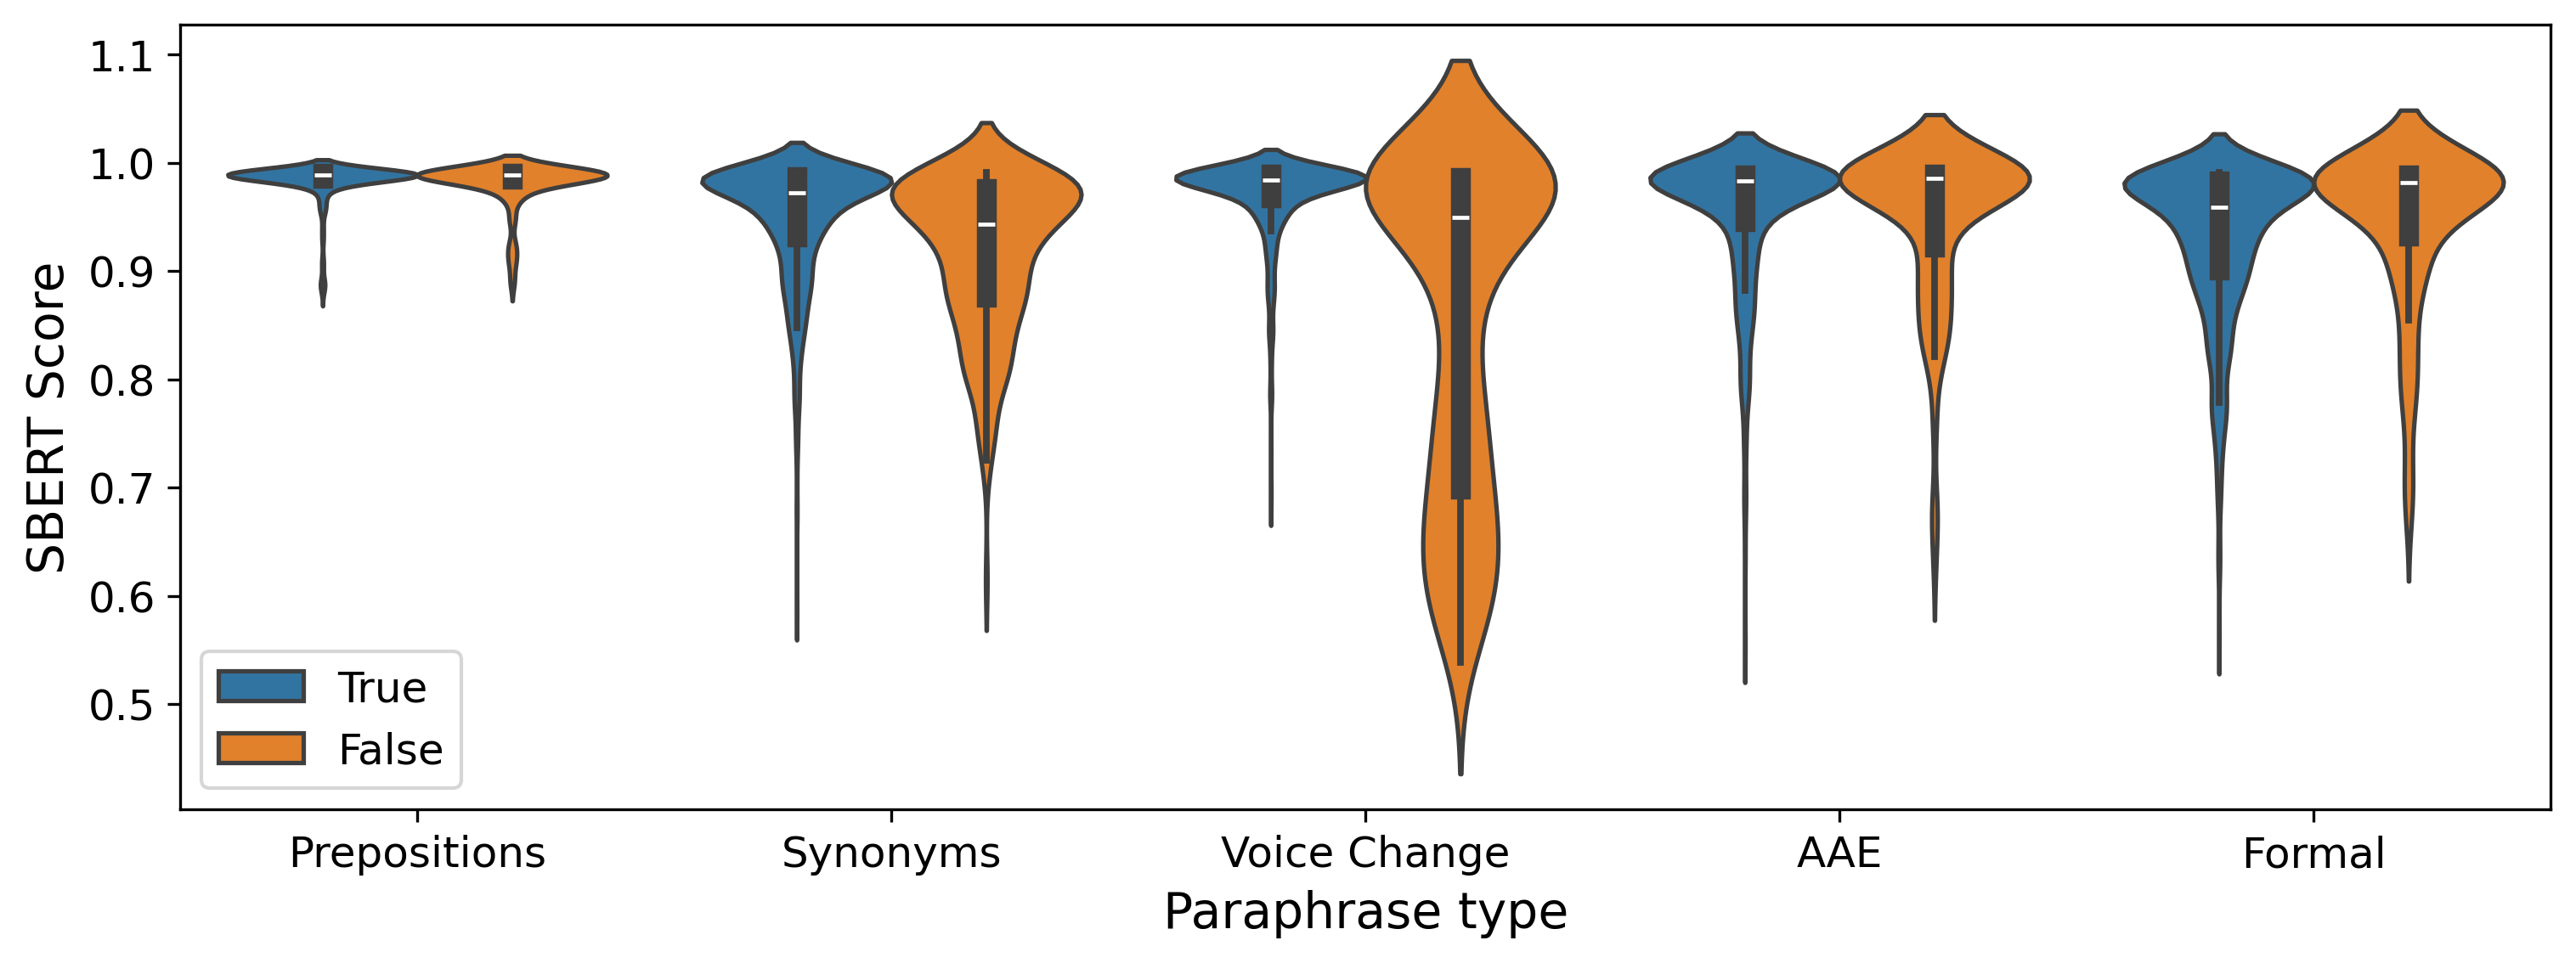}
            \caption{SBERT scores across paraphrase types.}
            \label{fig:violin-sbert}
\end{figure*}

\begin{figure*}[t]
\centering
        \includegraphics[width=\linewidth]{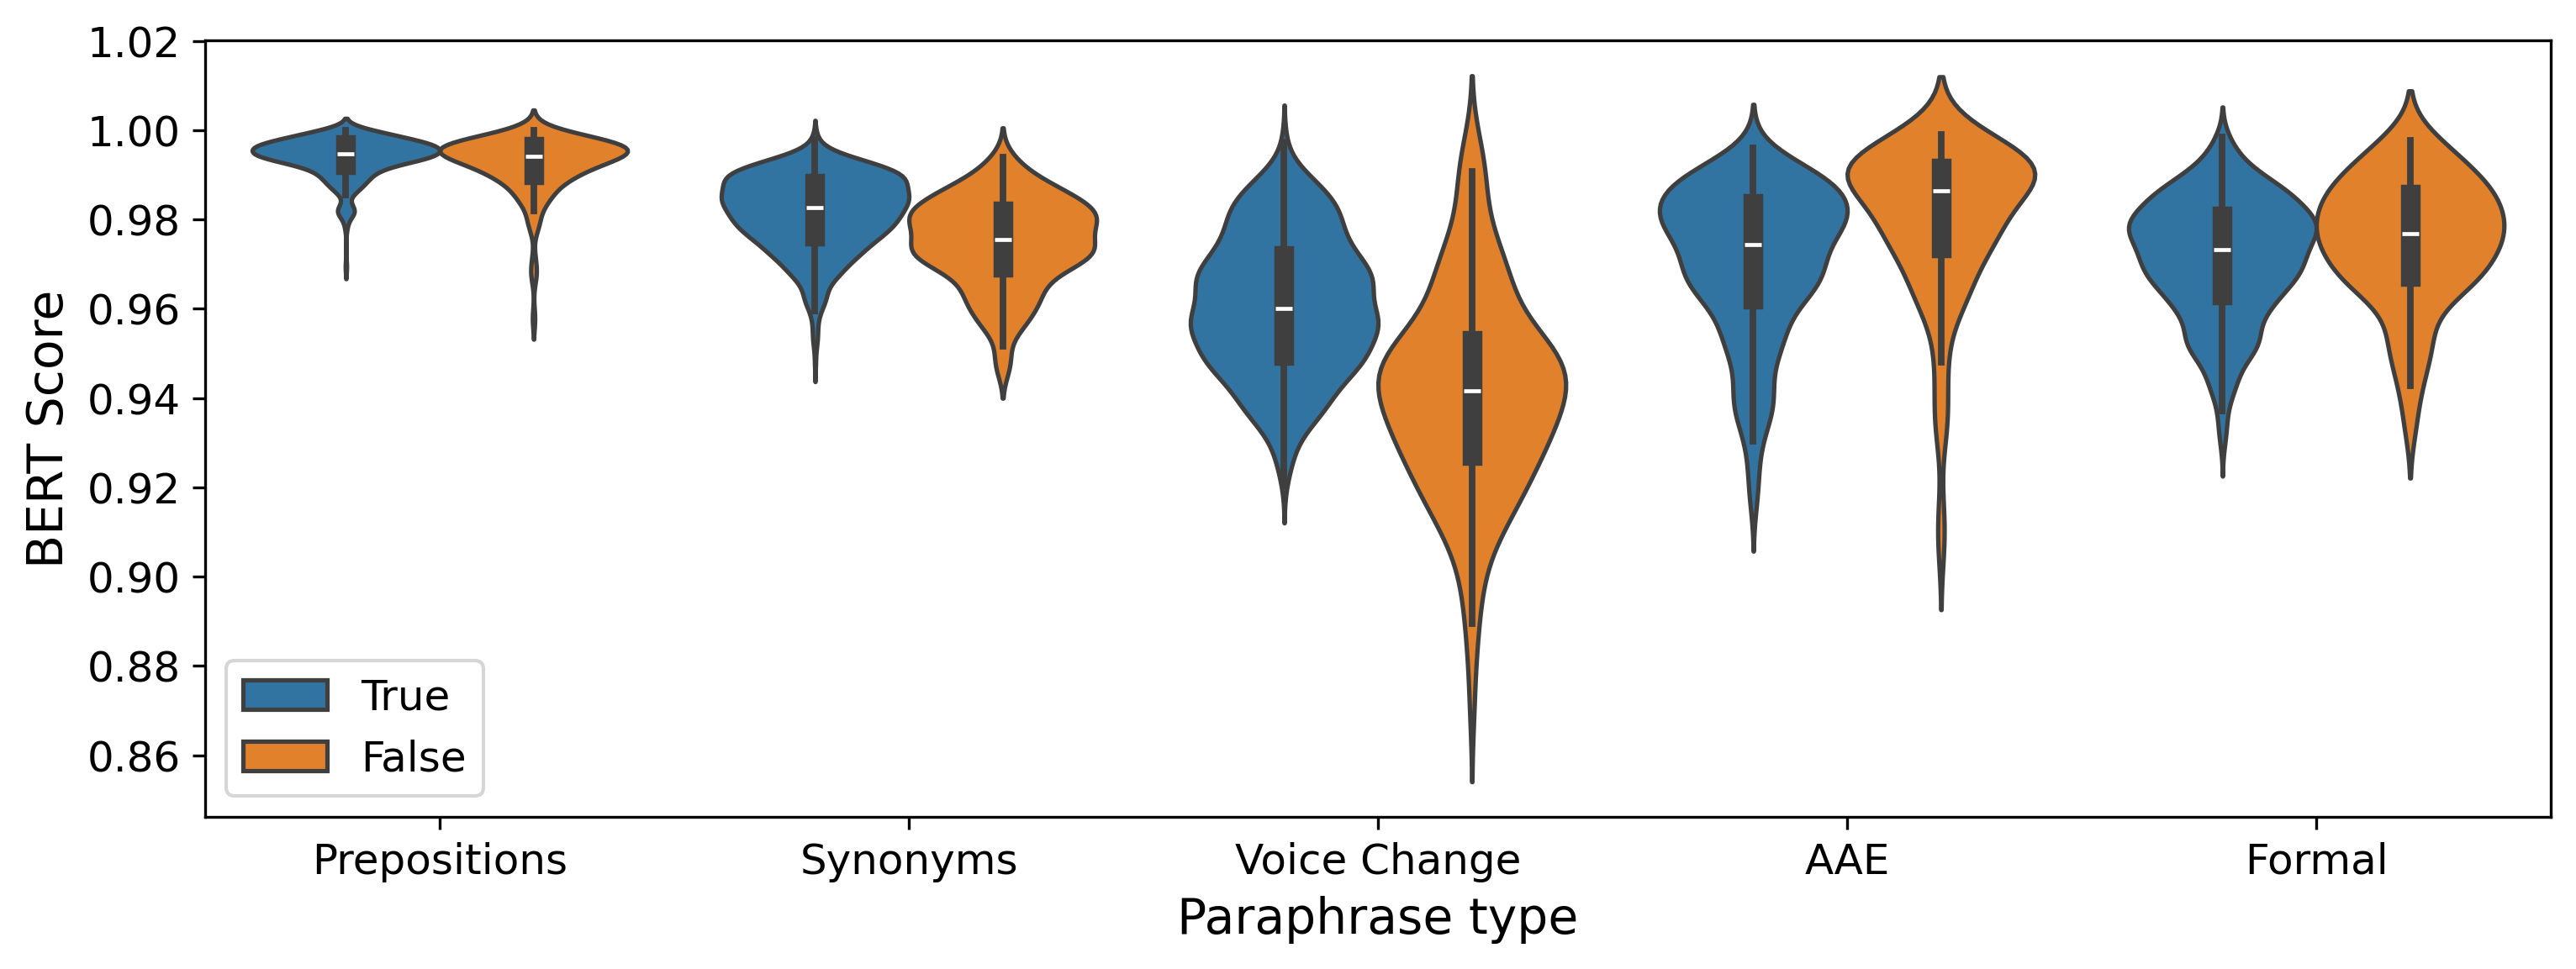}
            \caption{BERT scores across paraphrase types.}
            \label{fig:violin-bert}
\end{figure*}

\begin{figure*}[t]
\centering
        \includegraphics[width=\linewidth]{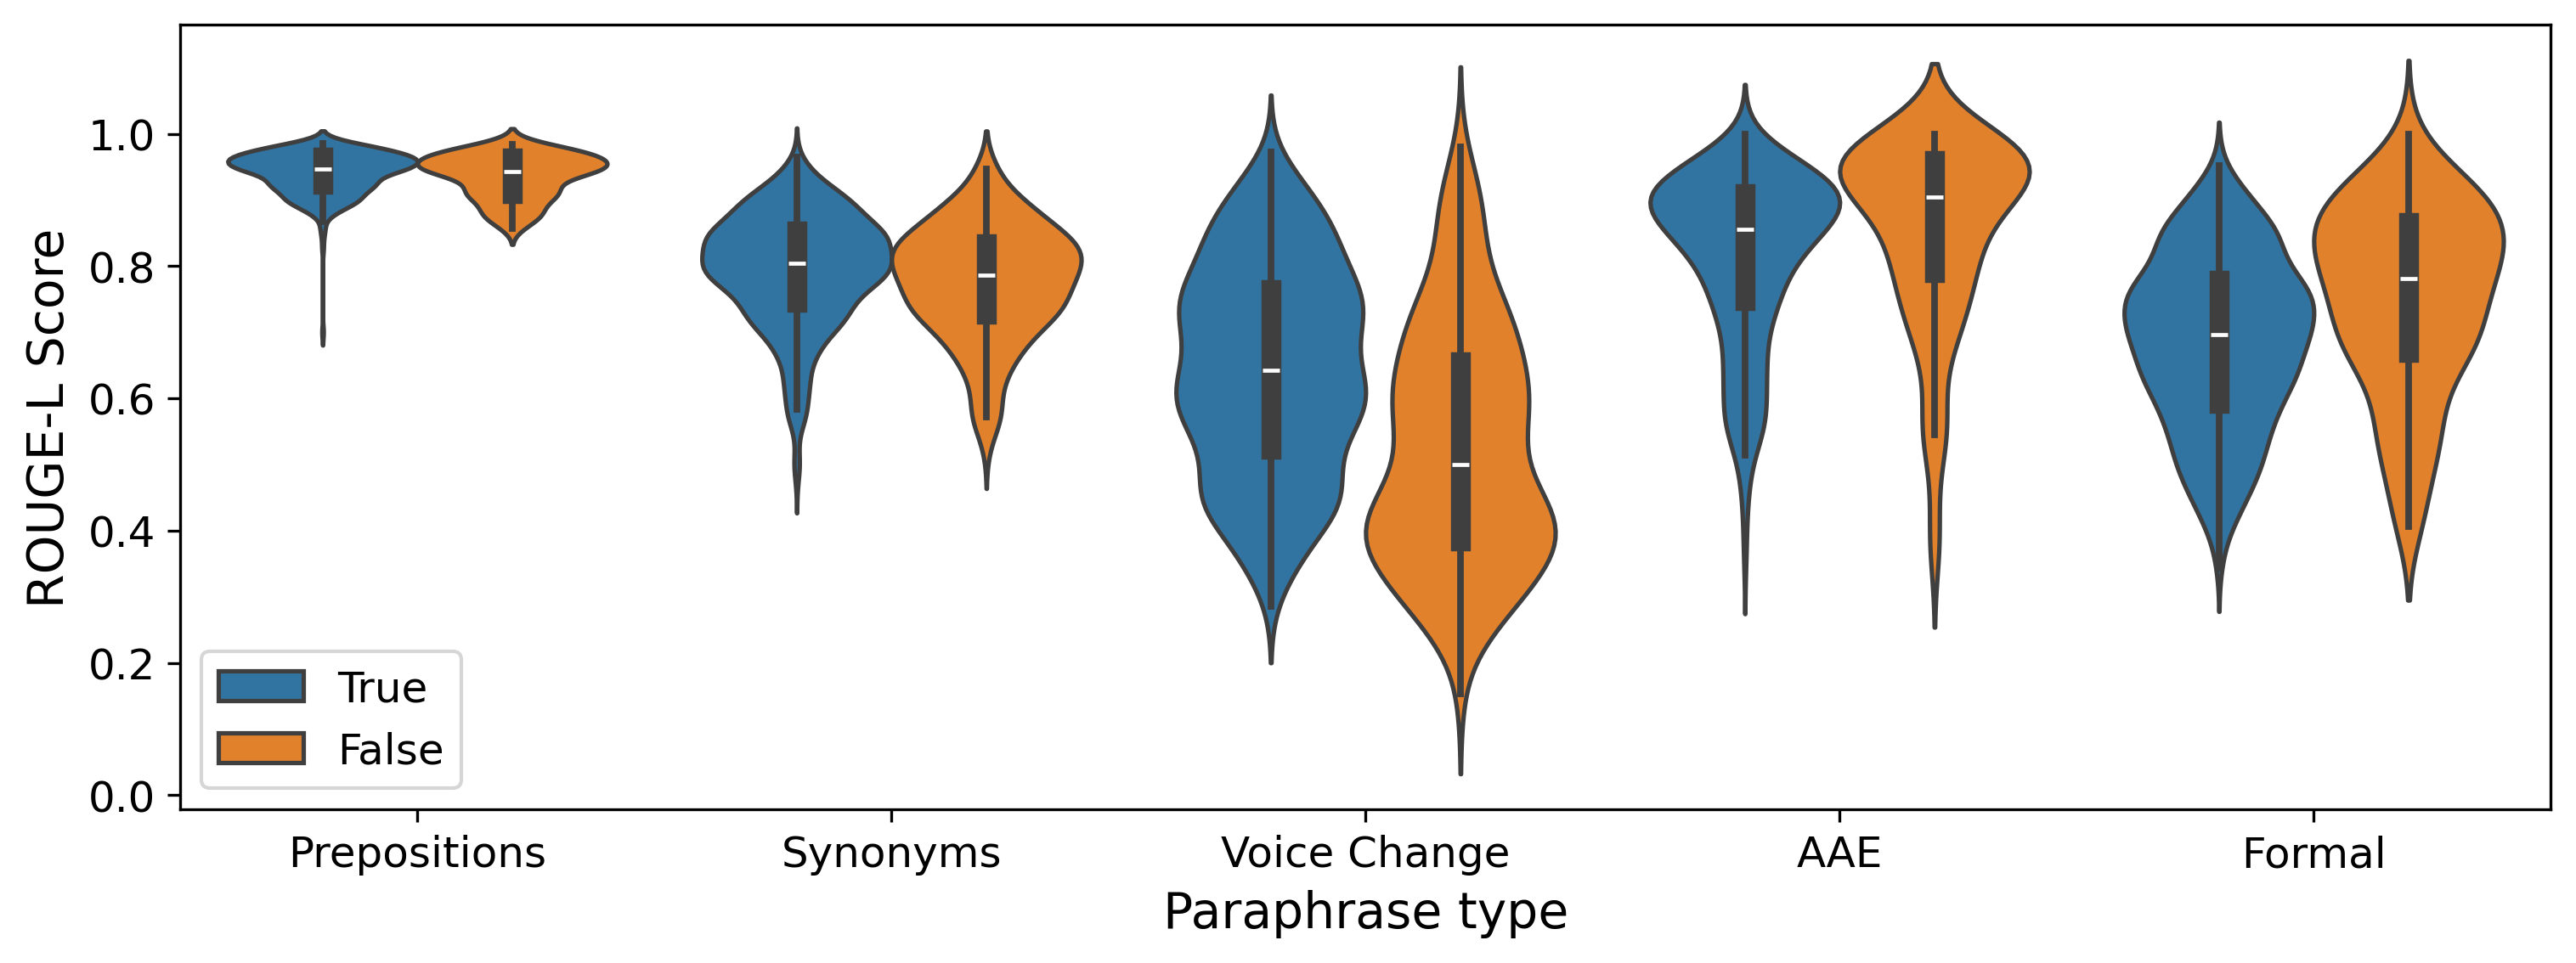}
            \caption{ROUGE-L scores across paraphrase types.}
            \label{fig:violin-rouge}
\end{figure*}

\begin{figure*}[t]
\centering
        \includegraphics[width=\linewidth]{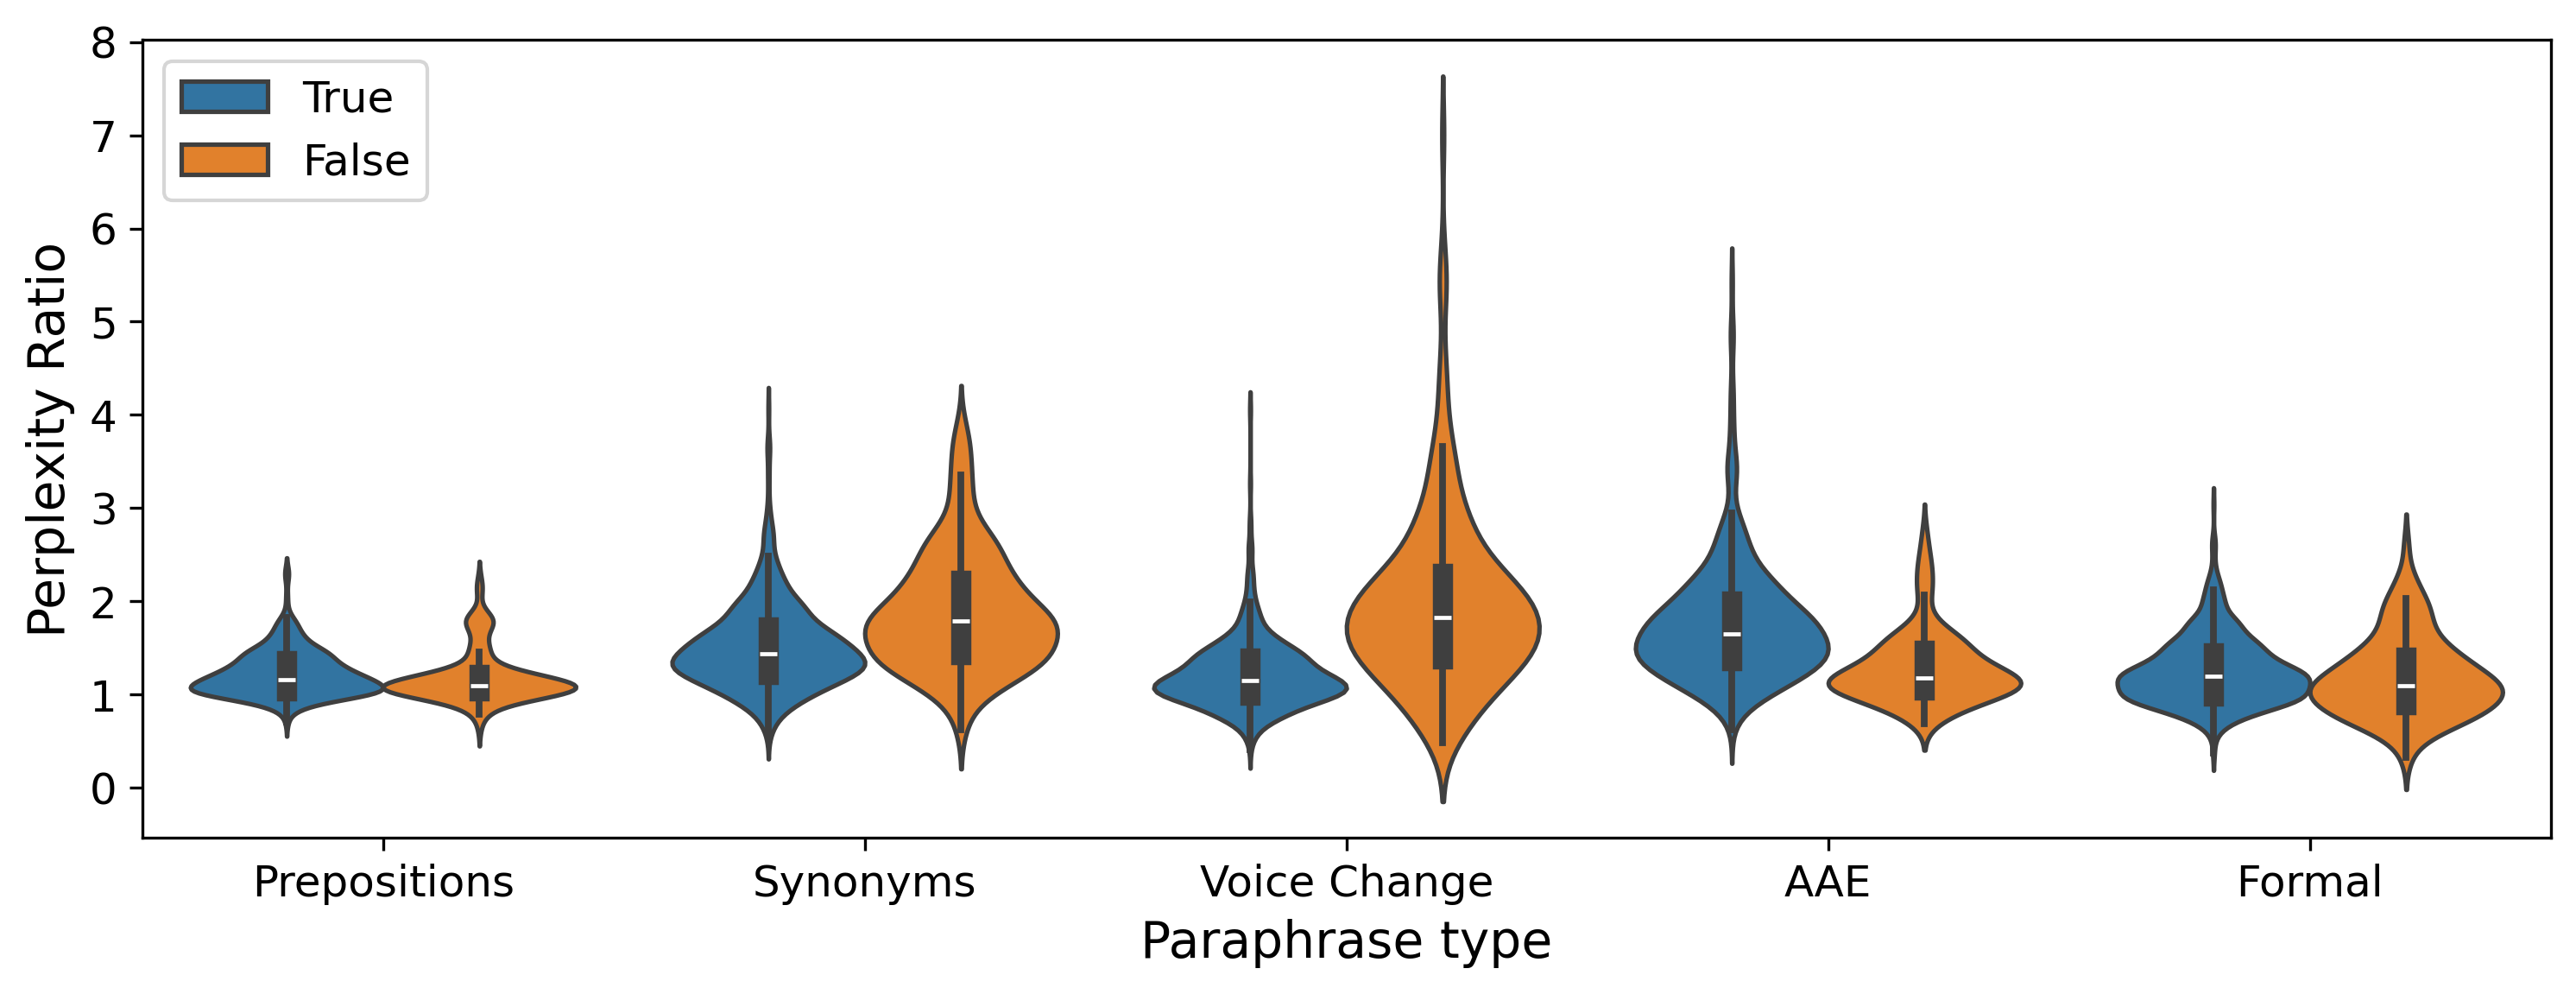}
            \caption{Perplexity Ratio across paraphrase types.}
            \label{fig:violin-ppl}
\end{figure*}
